# Supplementary material for: A Decentralized Framework for Serverless Edge Computing in the Internet of Things
Source: arXiv:2110.10974 source file (2021-10-21)
Supplement: Supplementary file 1 [file appendix.tex]

\newpage
\appendix

\setcounter{figure}{0}
\setcounter{table}{0}

\vspace*{\fill}
\begin{center}
{\large \textbf{Supplementary material}}
\end{center}
\vspace*{\fill}

\tableofcontents
\vspace*{\fill}

{\small%
\noindent%
\begin{tabularx}{\textwidth}{lX}
  DOI: & 10.1109/TNSM.2020.3023305 \\
  Title: & A Decentralized Framework for Serverless Edge Computing in the Internet of Things \\
  Authors: & \textit{Claudio Cicconetti, Marco Conti, \& Andrea Passarella} \\
  & Institute of Informatics and Telematics --- CNR --- Italy \\
  Publication: & IEEE Trans. on Network and Service Management \\
\end{tabularx}
}

\newpage

\section{ETSI MEC integration}
\myfigfulleps%
{etsimec_mapping}%
{ETSI MEC reference architecture (left) and mapping of the proposed components for serverless edge computing (right).}

\ac{ETSI} has standardized an
architecture and a suite of protocols for the realization of the
edge computing concept in a \ac{3GPP} access network such as \ac{LTE}
under the name of \ac{MEC}.
Indeed, the ETSI MEC is not part of the 3GPP specifications, but
it is likely that some key contributions will eventually converge
in such standards; furthermore, we note that the acronym ``MEC''
was initially intended for Mobile Edge Computing, but later changed
to Multi-Access Edge Computing to underline that the proposed
architecture might be applicable also to non-mobile wireless networks,
even though the standardization process has been heavily influenced
by this specific use case\footnote{Public announcement in Issue 2
of \ac{ETSI} newsletter 2017.}.
The ongoing definition of the standard has spurred several scientific
contributions, mostly focused on the virtualization and orchestration
challenges, especially related to the mobility of
\acp{UT}~\cite{Taleb2017a}.

We illustrate the main components of the \ac{ETSI} \ac{MEC} reference
architecture in the left part of \rfig{etsimec_mapping}, also showing
the names of the open interfaces defined in the specifications.
The system consists of three main entities: the user, who enters
the system via a \ac{UE} application; the \ac{MEH}, which is the
edge device hosting the \ac{ME} applications and services; the
platform, which is the set of back-end services managing the edge
computing resources and offering a single entry point to the \ac{UE}
applications.
More specifically, the reference architecture assumes that the
\acp{MEH} have a virtualized infrastructure for communication,
computation, and storage, which is managed by the \ac{VIM} in the
platform.
The \ac{ME} applications and services run as \acp{VM} on this
infrastructure: the former are counter-parts of the \ac{UE}
applications and can be enabled by the users through the \texttt{Mx2}
interface via an \ac{UE} application \ac{LCM} proxy; the latter,
i.e., the services, provide the local \ac{ME} applications with
features that can be exploited to provide the user with an enhanced
\ac{QoE}.

The standard specifies some \ac{ME} services that may be offered
by \ac{ETSI} \ac{MEC} compliant \ac{ME} platforms, e.g., for
reconfiguring the underlying routes of data flows related to the
application or for accessing radio network information or localization
information, but vendors are allowed to define further proprietary
services for market differentiation.
For the same reason, among all the interfaces referenced in the
architecture, only the \texttt{Mx2} and \texttt{Mp1} interfaces are
fully specified, while the rest are defined only in terms of their
high-level functions or, in some cases, technical requirements.
This choice is a compromise between free market competition and
ease of interoperability, and it implicitly defines exactly three
actors in the ecosystem: the \ac{UE} application developers; the
\ac{ME} application developers; the \ac{ME} platform providers.

In the right part of~\rfig{etsimec_mapping} we position the serverless
edge computing components proposed in \rsec{contribution} above in the
\ac{ETSI} \ac{MEC} reference architecture.
First, e-computers and e-routers can be materialized as \ac{ME}
applications within \acp{MEH}: there will be exactly one e-router
per \ac{MEH}, while the number and type of e-computers depend on
a periodic optimization process that loads/unloads applications
depending on the HW/SW constraints and the current (or forecast)
popularity of the applications.
The latter is equivalent to the function performed by the mobile
edge orchestrator in a traditional \ac{ETSI} \ac{MEC} system, and
it is not elaborated further in this work.
The e-controller, which must be aware of the location and capabilities
of all the e-computers and e-routers, is best positioned in the
\ac{MEPM}, which is a logically centralized entity with a global
view on the edge computing domain.
The \ac{SDN} controller is part of the \ac{VIM}.
In the figure we also show the data and control plane interactions
between the serverless edge computing entities.
As can be seen, consistently with the proposed decentralized
approach, the \ac{UE} application, residing on the \ac{IoT} device,
never interacts with the platform on the data plane.

Our work-in-progress \textit{open source} implementation of the \ac{ETSI}
\ac{MEC} \acp{API} to support serverless computing is available
on GitHub\footnote{\url{https://github.com/ccicconetti/etsimec}}.

\section{Avoiding loops in the hierarchical overlay}
\myfigeps[scale=1]%
{scalability-final}%
{Example showing a forwarding loop.}

\myfigeps[scale=1]%
{scalability-final-right}%
{Solution to the problem in~\rfig{scalability-final}. The entries with $^*$ are final.}

In the example in~\rfig{scalability-arch} there is no ambiguity
regarding the destination, because lambda requests arriving at E
are always forwarded to C, which has no other choice than sending
them to A.
However, let us consider now the example in~\rfig{scalability-final},
where each e-router (B or C) has the option to either send a
lambda request to an e-computer directly (A or D, resp.) or to
a peer e-router (C or B, resp.).
This may create a loop in the forwarding, causing the same lambda
request to be bounced between B and C, which is clearly to be
avoided at all cost.

A simple, yet effective, solution is that the e-controller
differentiates between destinations that reach directly an e-computer,
which we call \textit{final}, and those that reach an e-router
instead, which we call \textit{intermediate}.
Furthermore, we need a flag in the lambda request specifying
whether the request comes from a client or another e-router.
This way, each e-router has to restrict the destination selection
only to the final destinations if a request comes from an e-router,
but the same algorithms in~\rsec{algorithms} can be used without
other modifications.
The example with correct e-tables is shown
in~\rfig{scalability-final-right}, where two correct data paths
exist from a client accessing via e-router B\@: one to the e-computer
A via e-router B, another to the e-computer D via e-routers B and
C.

\section{Performance evaluation (further results)}

In this section we report the results from two scenarios aimed
at evaluating the following basic properties of the solution proposed:

\begin{itemize}[leftmargin=*,label={--}]
  \item Our fairness notion (see~\rsec{algorithms:destination}) is
  highly related to an efficient load balancing among e-computers.
  This is shown in a \textit{line topology} (\rsec{eval:line}) with a single e-router
  having ample choice of destination among many e-computers.
  Specifically, in these conditions LI, which is the most unfair of
  the three algorithms studied, is not even reported because it
  exhibits very poor performance, whereas RR, which enjoys both
  short- and long-term fairness, achieves best results in terms of
  delay.

  \item Network congestion is tackled efficiently by exploiting a
  cross-layer interaction with the \ac{SDN} controller (top branch
  of \req{weightupdate}), as illustrated in a \textit{ring tree
  topology} (\rsec{eval:ring}).

  \item Our solution is efficient in edge-cloud scenarios. This is
  shown in a \textit{pods topology} (\rsec{eval:pods}), where the e-routers automatically
  prefer remote (powerful) e-computers or nearby (low-power) devices,
  depending on their instantaneous load conditions, always aiming
  at reducing the latency of lambda responses.
\end{itemize}

We then conclude the extra results in the appendix with a scenario
in a \textit{tree topology} (\rsec{eval:tree}) that exacerbates the
effect on delay with hierarchical vs.\ flat forwarding, already
visible in \rsec{eval:large}.

Some of the results in this section have already been presented in
in~\cite{Cicconetti2018}.

\myssec{Emulator}{eval:emulator}
In this section we describe the emulator implemented.

\myfigeps[width=3.2in]{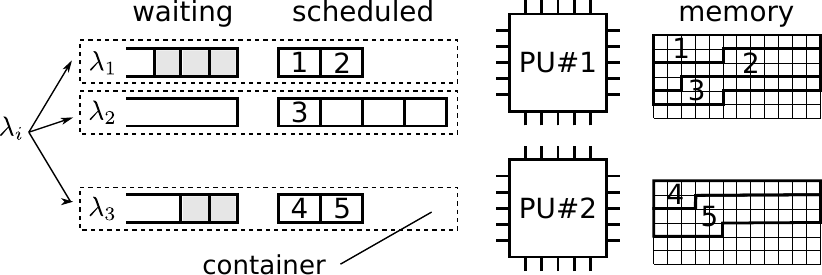}{Edge computer model used in the performance evaluation.}

Edge computers are emulated by means of user-space processes that
respond to lambda function activation requests with dummy responses
after a simulated \textit{execution time} that depends on the current
e-computer load.
The model realized by each e-computer is illustrated in
\rfig{edgecomputermodel}.
As can be seen, an e-computer is associated to physical resources,
i.e., \acp{PU} and memory, and logical resources, i.e., containers
hosting a number of workers.
Each container is specific for a given lambda function and only
executes on a given \ac{PU}, which, in turn, can access exclusively
a given memory bank.
When a client issues a lambda request it also specifies the
\textit{input size}.  In our analysis, we assume that the number
of operations required for the execution of $\lambda_i$ with input
size $N$ on a given \ac{PU} $j$ is:
\begin{equation}
\label{eq:numops}
n_{OP}(\lambda_i, N) = a_j + b_j \cdot N
\end{equation}
where $a_j$ takes into account the preparation for the execution
of the function, including, e.g., loading the required libraries
and drivers in the run-time environment, and $b_j$ is a proportional
factor that models a $\mathcal{O}(N)$ time complexity of the algorithm
being run.
Quite clearly, such an assumption is not valid for \textit{any}
algorithm or application, but we deem it sufficient to capture
heterogeneous needs for the same function being run by different
clients or by the same client at different times.
Likewise, the memory required by the execution of $\lambda_i$ with
input size $N$ on \ac{PU} $j$ is:
\begin{equation}
\label{eq:memory}
n_{MEM}(\lambda_i, N) = c_j + d_j \cdot N
\end{equation}
Different models for the number of operations and memory requirements
of lambda functions can be easily accommodated in our software and
we plan to expand the analysis to encompass such additional degrees
of freedom in a future study.

As a new lambda request arrives at an e-computer, first of all it
is directed to the serving container, which computes $n_{OP}$ and
$n_{MEM}$ according to \req{numops} and \req{memory}, respectively.
The request is then queued if either all the workers are busy or
it must be blocked because the memory requirements exceed the current
available memory.
In the latter case, no further lambda request is put in execution
until the blocked request is served by a worker.
This ensures that a \ac{FCFS} policy is observed and also prevents
starvation.
%
%Pre-emption and real-time scheduling policies are not implemented
%in the current version, but planned for later releases.
%
A queued lambda is served once a worker becomes free and there are
no earlier blocked lambdas.
A scheduler is implemented in the e-computer to dispatch lambda
function responses, where the dispatch time $T$ of $\lambda_i$ over
a period for which $W$ workers are active on \ac{PU} $j$ is:
\begin{equation}
\label{eq:lambdatime}
T(\lambda_i) = n_{OP}(\lambda_i) \cdot \frac{S_j}{W}
\end{equation}
where $S_j$ is the speed, in number of operations per seconds, of
\ac{PU} $j$.
%
% In later releases we plan to implement more sophisticated scheduling
% policies, including preemptive algorithms to better support tasks
% with an associated priority and backfilling with system-generated
% run-time estimates to increase throughput.
%
The \textit{load} of any \ac{PU} of an e-computer is monitored for
performance analysis reasons: it is defined as the ratio between
the sum of periods in which the \ac{PU} is busy and the measurement
interval (in other words, load 1 means that the \ac{PU} is continuously
busy with execution of some lambdas whereas load 0 means a completely
idle \ac{PU}).

\myssec{Line topology}{eval:line}
\myfigeps[width=2.5in]{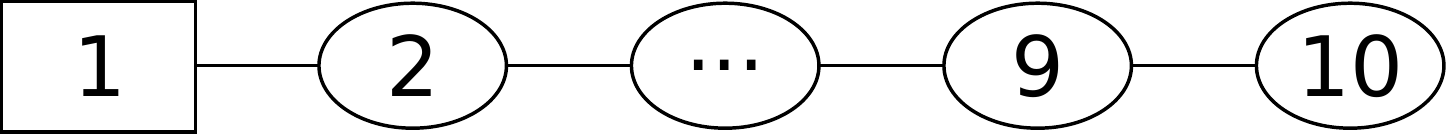}{Line topology.}

In this batch of experiments we have 10 edge nodes connected in a
line topology, see~\rfig{lineartopo}: all the clients access edge
computing functions via a single e-router that is located in node
1, while all the other nodes act as \textit{constrained-device}
e-computers.
The $a_j$ and $b_j$ values in \req{numops} are set as in
\rsec{eval:ring}.

We use two link models: \textit{ideal link}, where we let Mininet push packets between emulated networking devices as fast as allowed by the host (roughly 30~Gb/s with the server used), and \textit{real link}, where communication is constrained by a token bucket allowing a 2~Mb/s rate with a 2~ms delay.
With a real link, we also simulate a network congestion mid-chain, i.e., between nodes 5 and 6, with background \ac{UDP} traffic unrelated to edge computing.
Every edge client issues lambda requests of constant size equal to 200~bytes at random intervals: the time between two consecutive requests is drawn from a uniform r.v.~in $[0, 2]$~s.
A single lambda request type is used by all the clients.

\myfigeps{linear-net}{Line topology: Total network traffic vs.\ number of edge clients, RR only.}

In \rfig{linear-net} we report the total network traffic as the number of clients increases from 10 to 180.
Without network congestion the traffic increases linearly with the number of clients.
We note that the ideal link curve lies on top of the real link curve because in the latter case the e-computers closer to the e-router tend to be used more, which spawns less traffic in the network.
On the other hand, with network congestion the traffic saturates above 80 clients because that is the maximum that can be handled by e-computers \textit{before} the congested link.
We only show the curves with RR since those obtained with RP are almost identical for each respective case.

\myfigeps{linear-out-95th}{Line topology: 95th percentile of latency vs.\ number of edge clients.}

In \rfig{linear-out-95th} we show the 95th percentile of the latency.
Let us consider the cases without congestion first.
With RR the curves are almost constant until 90 clients and they increase only slightly until 150 clients.
Performance drops significantly only with 180 clients, when the e-computers become overloaded (the average load per computer with 180 clients is very close to 1).
The latency difference between the ideal and real link cases is purely due to the difference of emulated link latency.
On the other hand, with RP, both ideal and real link curves increase significantly even at low loads.
This is because the random scheme sometimes creates load spikes by sending multiple lambda requests to the same e-computer even though there are others (almost) idle.
Such an effect is barely noticeable in the average delay or lower quantiles (both not shown), but quite prominent in high quantiles, which are important for jitter-sensitive \ac{IoT} applications.
Finally, with both RR and RP, the presence of a congested link severely degrades the performance except at very low loads.

%The load is increased until the all the e-computers are overloaded, which happens sooner in wtc2 case because of network congestion.
%
%\myfigeps{linear-util}{~}

\myfigeps{linear-util-70}{Line topology: Load of e-computers with 70 clients, RR only.}

In \rfig{linear-util-70} we show the average load of e-computers (numbered as in \rfig{lineartopo}) with 70 edge clients with RR\@.
As can be seen, with ideal link, the load is perfectly flat: with very small communication delays every e-computer is considered the same even though there are up to 9 hops to traverse to reach the right-most one in the chain.
With real link, the load decreases almost linearly since closer e-computers tend to be used more frequently.
With congestion, the load drops after the 5th e-computer, but remains well above zero also for the nodes after the congested link, which accounts for the poor performance shown in \rfig{linear-out-95th}.
These observations confirm that a forwarding scheme alone is not sufficient to handle (temporary) network congestion situations: while the effects could be reduced by tweaking the probe scheme parameters (for instance in these experiments we have an initial probe period of 1~s that might be increased), this would in turn increase the time required for recovering the use of the blacklisted e-computers after network congestion disappears.
On the other hand, a more robust and efficient solution is to exploit
information from the \ac{SDN} controller, as in~\req{weightupdate},
as evaluated later in~\rsec{eval:ring}.

\myssec{Pods topology}{eval:pods}
\myfigeps[width=3in]{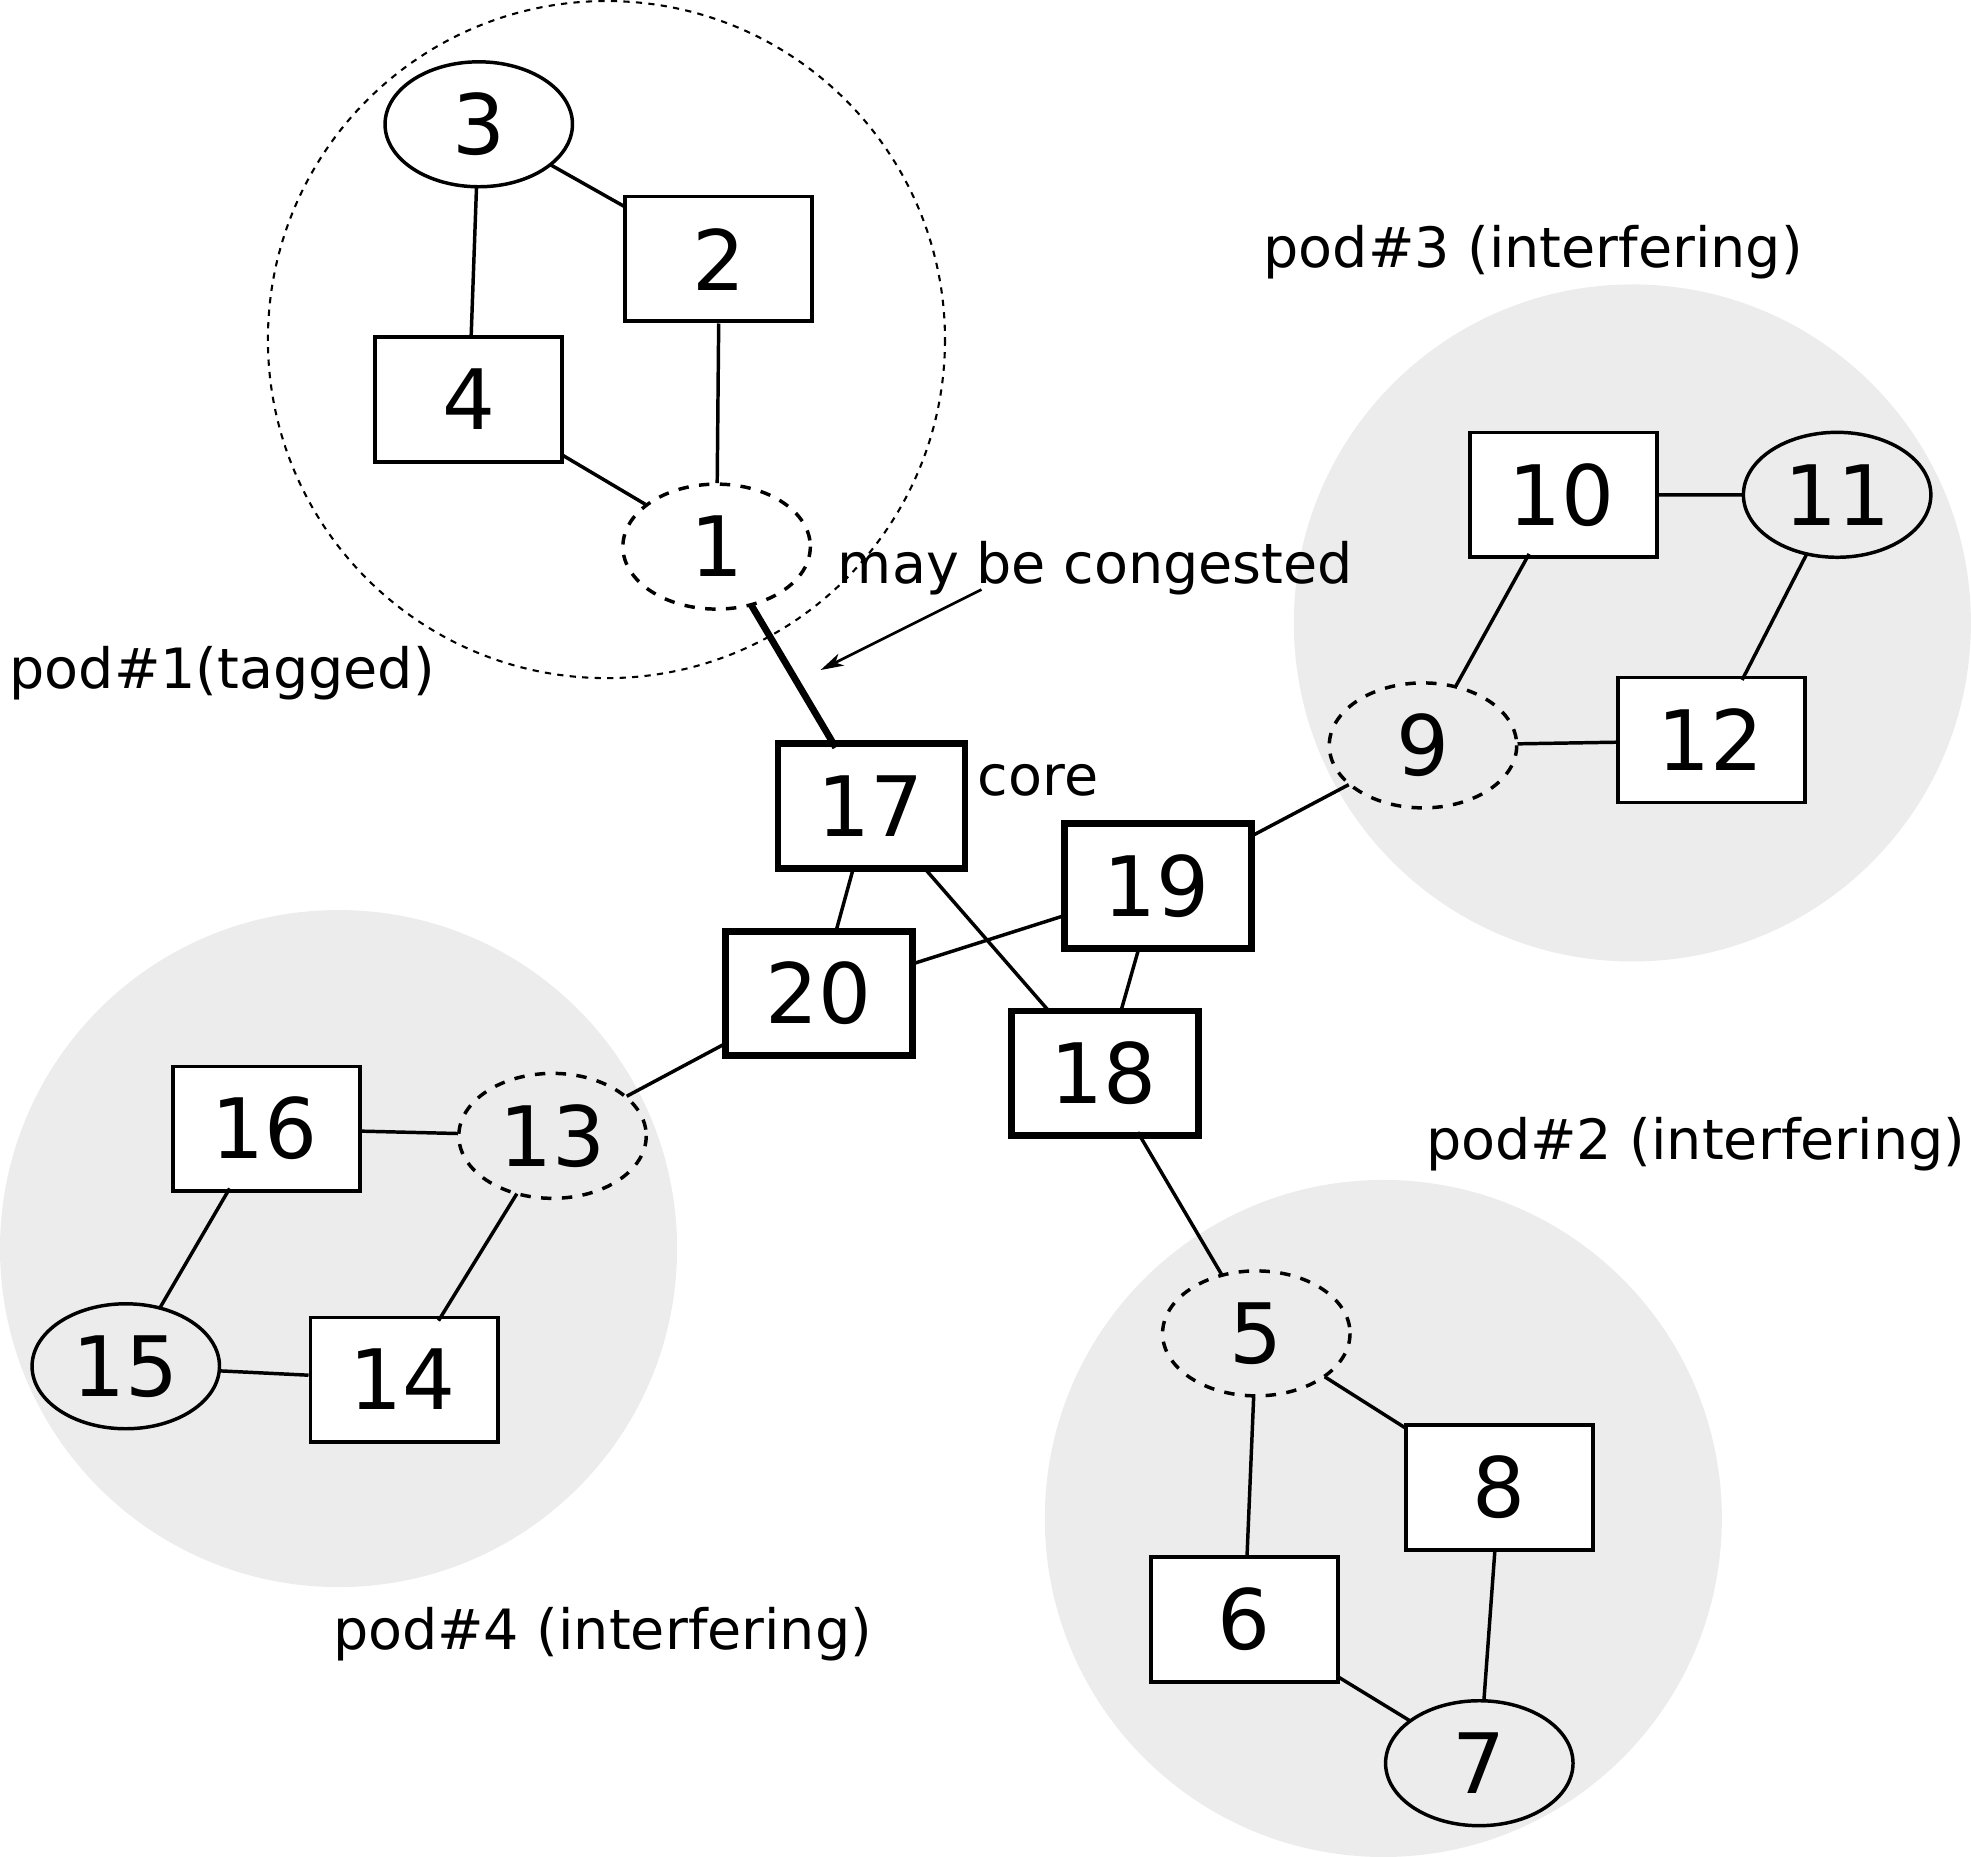}{Pods topology.}

In this scenario the nodes are arranged in four ``pods'' connected by a middle ``core'', see \rfig{podtopo}, to mimic real \ac{MBWA} deployments in urban scenarios.
Like in the previous scenario, we have emulated \textit{ideal} vs.\ \textit{real} links with Mininet.
%We have emulated links with Mininet in the \textit{real} configuration only.
Even-numbered nodes in each pod act as \textit{constrained-device} e-computers, all the nodes in the core (from 17 to 20) act as \textit{full-server} e-computers, whereas clients connect to e-routers in the leaf nodes (3, 7, 11, 15).
The $a_j$ and $b_j$ values in \req{numops} are set as in \rsec{eval:ring}.
We have run three batches of experiments.

In the first batch of experiments the e-computers of a given pod can execute lambdas of a single type (i.e,~pod\#$i$ computers offer $\lambda_i$), while the e-computers in the core can execute all four types ($\lambda_1-\lambda_4$).

Five clients in pod\#1 are considered as ``tagged'' and they issue a random number of consecutive $\lambda_1$ requests, all with constant size equal to 200~bytes, drawn from a Poisson distribution with mean 5, every 2~s.
The clients on the other three pods are considered as ``interfering'' and they issue 1000-byte $\lambda_j$ requests (where $j$ is the pod index) at uniformly distributed random intervals in $[0, 0.5]$~s.
The number of interfering clients per pod is increased from 2 to 48.

 \myfigeps{pod-net-v1}{Pods topology (I): Total network traffic vs.\ number of interfering clients.}

In \rfig{pod-net-v1} we show the total network traffic as the number of interfering clients increases.
As can be seen, at low loads the curves increase proportionally because every new client added brings new lambda requests that consume network resources.
However, after 28 interfering clients per pod the traffic remains constant: after that point the e-computers handling lambda functions of interfering clients are overloaded, and adding new clients does not further increase the traffic.
As with the line topology, the ideal link curves lie respectively above the corresponding real link curves because with ideal communication the e-routers are more aggressive in dispatching execution of lambda functions on e-computers that are far away.
 
\myfigeps{pod-out-v1}{Pods topology (I): Latency of tagged vs.\ number of interfering clients.}

We report the latency, both mean and 95th percentile, in \rfig{pod-out-v1}.
Despite the system becoming increasingly saturated, the tagged clients, whose number remains constant, are protected from interference of clients in the other pods through the load balancing properties of the destination selection algorithms in the e-router.
More specifically, RR and RP yield similar performance in terms of the mean delay, but when the 95th percentile of delay is considered RR provides much better performance, especially before full saturation of interfering clients, i.e., before 28 interfering clients per pod.

\myfigeps{pod-out-v2}{Pods topology (II): Latency vs.\ number of interfering clients, RR only, real link only.}

The second batch of experiments is the same as the first, but all the e-computers in pods offer the lambda type required by the tagged clients, while the interfering clients may only exploit the e-computers in the core.
We only report the results with real link and RR forwarding scheme.

Latency is reported in \rfig{pod-out-v2}.
Also in this case the tagged clients are protected from harmful interference from clients in the other pods as their load increases.

\myfigeps{pod-util-v2}{Pods topology (II): Load per e-computer, RR only, real link only.}

It is interesting to analyze the latency results together with the load distribution, shown in \rfig{pod-util-v2}.
At low loads, i.e., below 20 interfering clients, until the latency curves are almost constant, only the core e-computers are used, since they are sufficient to serve both tagged and interfering clients and are much faster than the peripheral e-computers in the pods.
With 25 interfering clients things start to change: the load of core e-computers approaches 1, therefore the processing delays become significant even when lambdas are executed there; for this reason, the load of e-computers in pods rise.
The effect is even more prominent as the number of interfering clients increases further, and the load of core e-computers becomes 1.
Anyway, the load of nodes 2 and 4, which are closest to the e-router (located in node 3, see~\rfig{podtopo}, again) is higher than that of the e-computers in the other pods, due to their proximity.
 
In the third batch of experiments, we keep the number of interfering edge clients constant and equal to 5 on all pods, but inject a variable amount of background \ac{UDP} traffic between nodes 1 and 17 until link saturation.
Note that node 17 provides the tagged clients with access to the powerful e-computers in the core (see again \rfig{podtopo}).
We only report the results with RR destination selection.

\myfigeps{pod-out-v3}{Pods topology (III): Latency vs.\ background UDP traffic, RR only.}

We show the latency in \rfig{pod-out-v3}.
We note that since saturation occurs because of network conditions, rather than because of e-computers becoming overloaded like in the other batches of experiments in this section, the e-router in pod\#1 is not entitled to scrap away the destinations beyond the congested link since it has no way of knowing when communication with them will work normally again (remember up until this point we have disabled the upper branch in \req{weightupdate}).
As a result, the tagged clients are unprotected from network load spikes: as soon as the background \ac{UDP} traffic exceeds the link capacity, latency becomes very significant, especially in terms of high quantiles.

\myfigeps{pod-util-v3}{Pods topology (III): Load per e-computer, RR only.}

As a confirmation that edge computing load is not the root of such poor performance, we report in \rfig{pod-util-v3} the load distribution, showing that e-computers in the pod (not affected by link congestion) are far from being overloaded, while e-computers in the core are probed despite being (unknowingly to the e-router) affected by congestion.

\myssec{Ring tree topology}{eval:ring}
\myfigeps[width=2in]{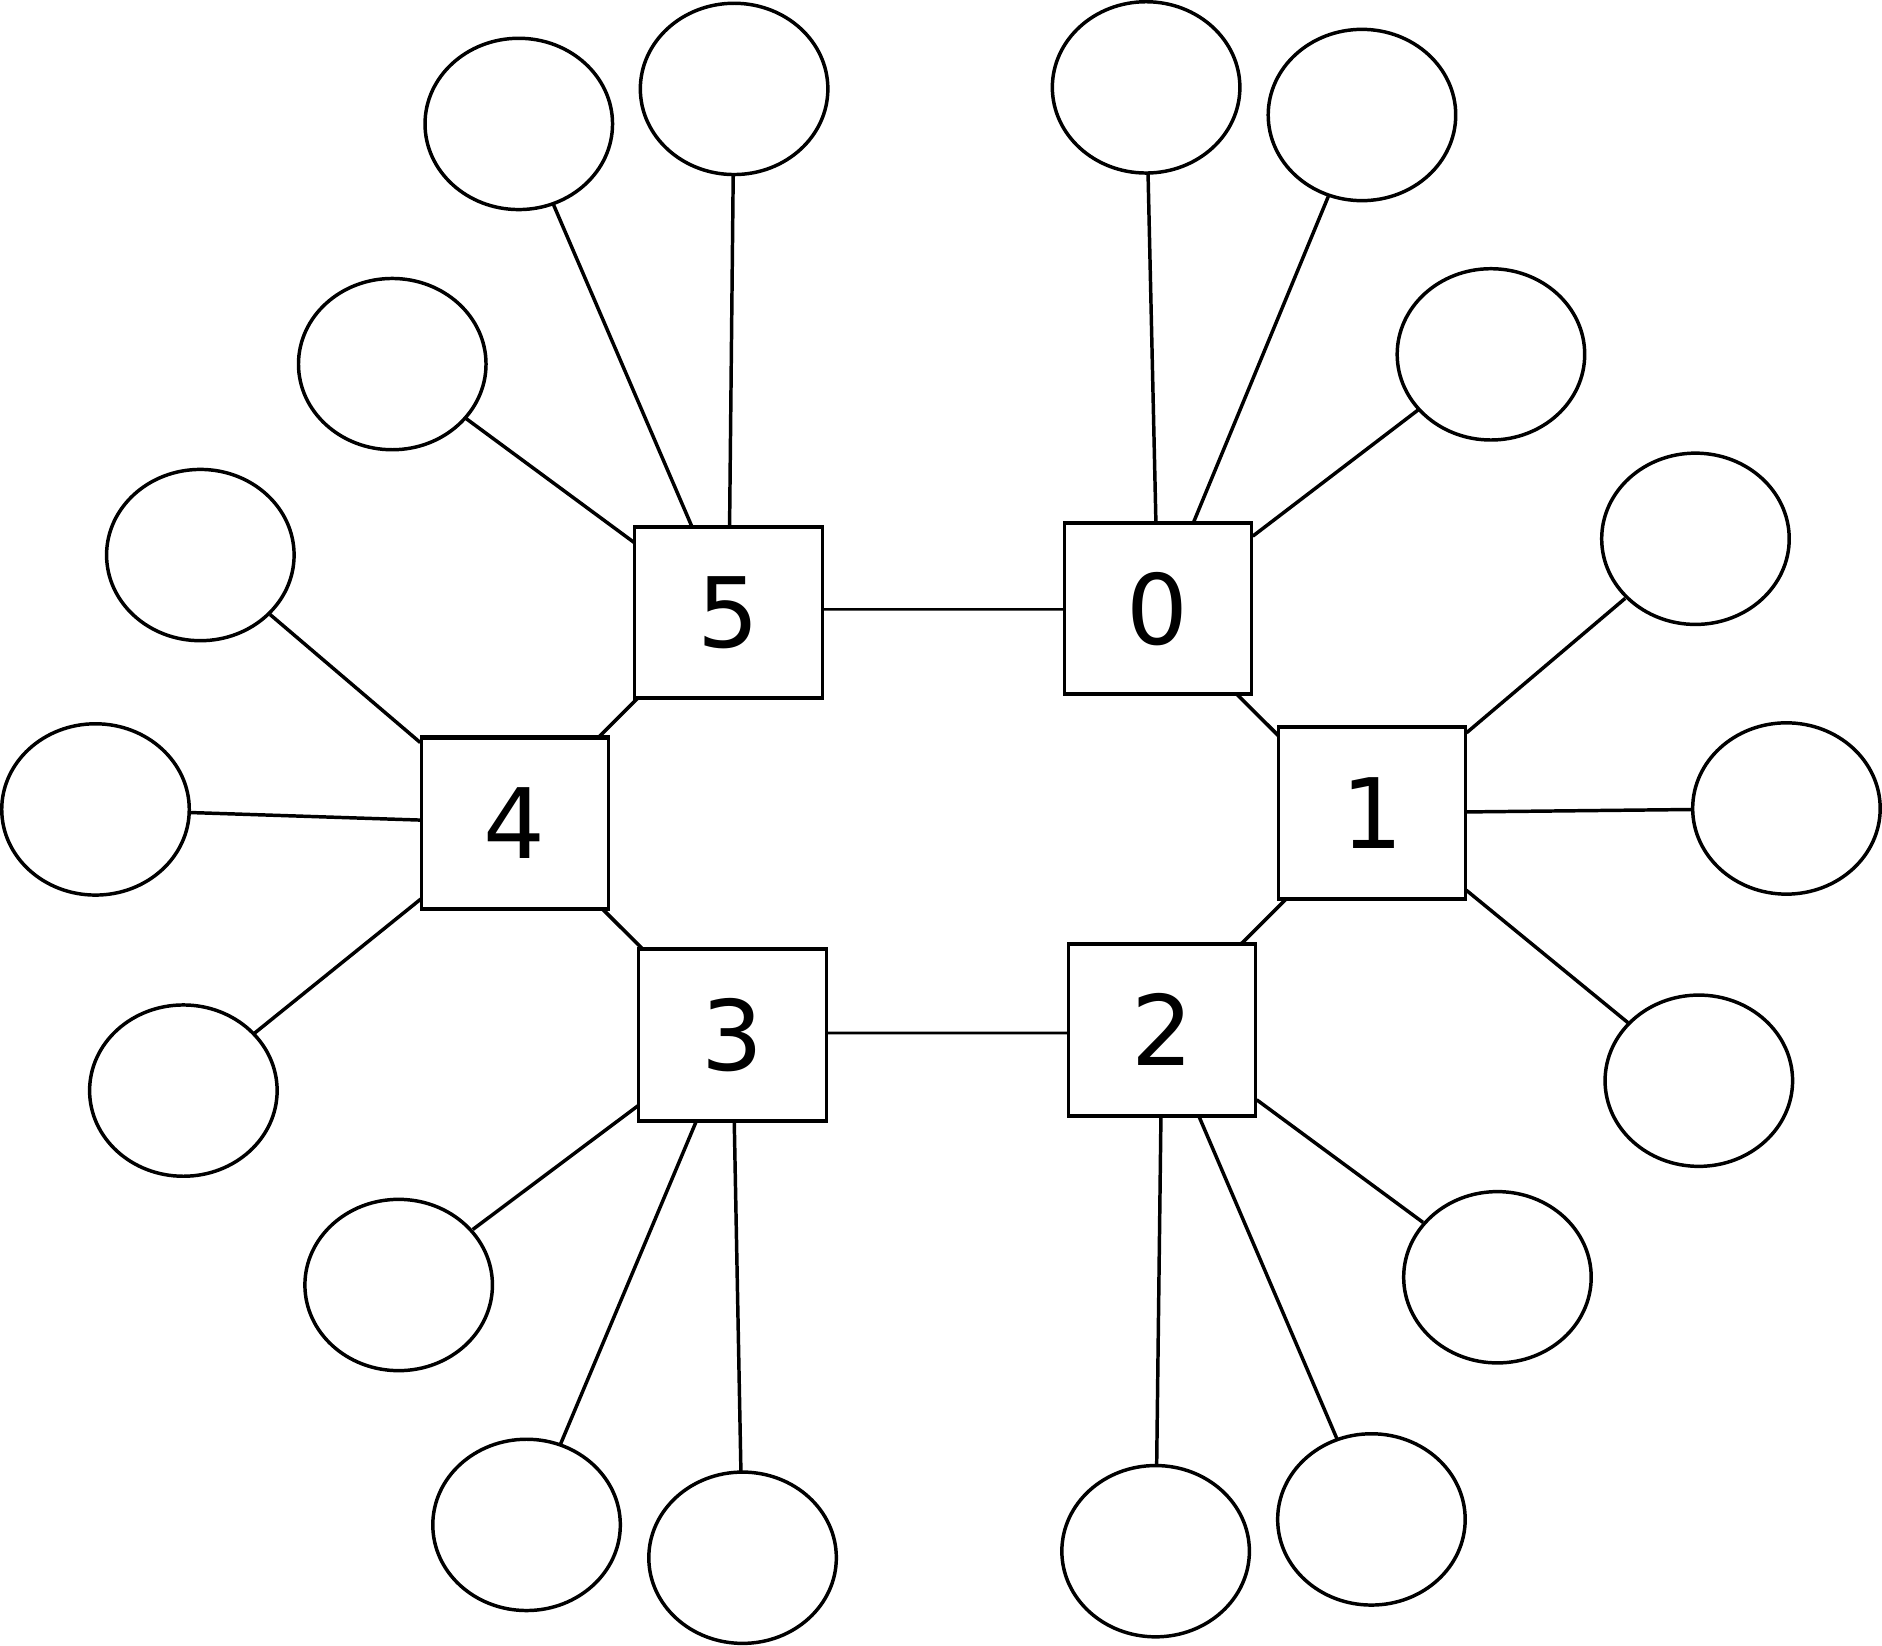}{Ring tree topology (\rsec{eval:ring}), with 6 nodes in the inner ring.}

In this scenario the nodes are arranged in a ``ring tree'' topology,
as illustrated in~\rfig{circtopo}: there is a core network of nodes
arranged in a ring, each sprouting a number of nodes.
All the inner ring nodes act as \textit{full-server} e-computers,
while all the other nodes in the outer tier act as e-routers.
The number of inner ring nodes is increased from 4 to 10 (it is 6
in~\rfig{circtopo}).
Each ring node always has 3 leaf nodes.
The communication links are constrained by a token bucket allowing
a 2~Mb/s rate with a 2~ms latency.
The parameters in \req{numops} are set as $a_j = 4\cdot10^6$ and
$b_j = 10^6$, with input size of lambda requests ranging from
200~bytes to 2000~bytes, which gives an execution duration ranging
from 1.3~ms to 12.5~ms provided that there is no other concurrent
task running.
The input size is variable because we are interested in evaluating
the latency properties of the weight updating and destination
selection algorithms with different processing times.

In this scenario we focus on a network whose edge computing traffic
is light to show the benefits of using extra information available
at the \ac{SDN} controller to influence destination selection
strategies.
Each e-router has a single edge client that issues lambda requests
according to an \ac{IPP}: ON and OFF phases alternate, where lambda
requests of size drawn from a uniform r.v.\ in $[200, 2000]$~bytes
are generated only during the ON phases, with a random pause between
requests drawn from a uniform r.v.\ in $[0.1, 0.5]$~s; the duration
of the ON and OFF phases is drawn from exponentially distributed
r.v.'s with mean 5~s and 20~s, respectively.
Furthermore, background \ac{UDP} traffic is generated periodically
between nodes $i$ and $i+1$: no background traffic for 20 seconds,
background traffic from 1 to 2 for 20 seconds, no background traffic
for 20 seconds, background traffic from 2 to 3 for 20 seconds,
etc\@.

First we show the mean latency in \rfig{circular-out-histo}.
For all ring sizes the latency is much smaller when the \ac{SDN} congestion detection mechanism is enabled, with slight differences among the different forwarding schemes.
If the \ac{SDN} congestion detection mechanism is disabled RP exhibits worst performance: this is because both RR and LI embed a mild form of protection against bad e-computer destinations, even though neither of them is sufficient.

\myfigeps{circular-out-histo}{Ring tree topology: Mean latency as the network size increases.}

The average load of e-computers is reported in \rfig{circular-util-histo}.

\myfigeps{circular-util-histo}{Histogram of the average load of e-computers.}

The cumulative distribution of the latency, for the only case of 10 nodes in the inner ring, is shown in \rfig{circular-out-cdf}.
As can be seen, with congestion detection the RR curve lies above that of both RP and LI, which achieve similar performance to one another.
Without congestion detection, despite the reasonable performance in terms of the mean delay, the jitter (i.e., high quantiles of delay) is compromised with all destination selection algorithms.

\myfigeps{circular-out-cdf}{%
Ring tree topology: CDF of latency with inner ring size = 10 nodes.}

\myssec{Tree topology}{eval:tree}
\myfigeps[width=2in]{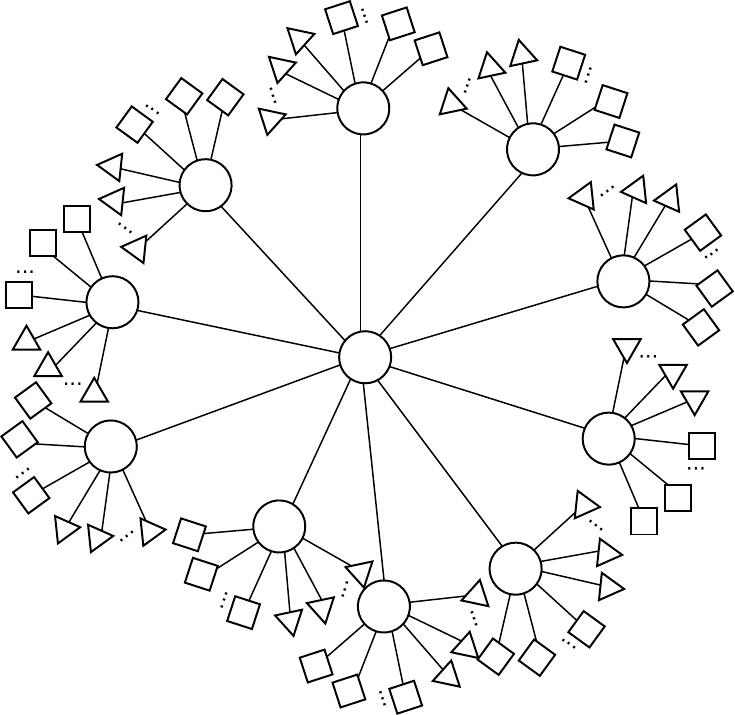}{Tree topology.}

In this section we use the topology in~\rfig{treetopo} to investigate
the impact of using a two-tier overlay, as described in~\rsec{scalability},
in a regular layout consisting of a 10 e-routers connected to a
central node via fast links (100~Mb/s, 1~$\mu$s latency), emulating
a backhaul network, while the e-routers, in turn, acts as a ``gateway''
to 10 further edge nodes and a variable number of clients each via slightly
slower links (25~Mb/s, 100~$\mu$s latency).
The $a_j$ and $b_j$ values in \req{numops} are set as in
\rsec{eval:large}.
In this layout with a two-tier overlay the home e-router of every
e-computer is always its own gateway.
We increase the total number of clients from 40 to 200, while the
number of e-computers is constant and equal to 100.

The average size of the e-tables is $14 \pm 3.1$ when using a
two-tier overlay, while it is always 100 with a flat overlay.
In every run, we drop randomly the e-computers on the 10$\times$10
leaf edge nodes and we associate randomly the clients to e-routers
and such association does not change for the whole duration of the
experiment.
During the experiment all clients continuously repeat the execution
of the same lambda request, thus the total number of lambda executions
may vary per configuration.

\myfigeps{tree-delay}{Tree topology: mean and 99th percentile of delay.}

In~\rfig{tree-delay} we show the mean and 99th percentile of the delay.
As in~\rsec{eval:large} we can see that the delay with a two-tier
scheme is smaller than that with a flat scheme.
This becomes more evident at high loads and when considering the
99th percentile compared to the average.
%
%With all the traffic loads, with a two-tier scheme the average
%number of hops, on the serverless overlay plane, was between 2.4
%and 2.5 (with a flat scheme it is always 2 by design).

% \myfigeps{tree-tpt}{Tree topology: total network throughput.}
